# Supplementary material for: Quantum back-action evading measurement of collective mechanical modes
Source: arXiv:1608.06152 ancillary file (2016-09-27)
Supplement: Supplementary file 1 [file TwoModeBAE_Supplement.pdf]

# Supplemental Material for "Quantum back-action evading measurement of collective mechanical modes"

C. F. Ockeloen-Korppi,[1] E. Damskägg,[1] J.-M. Pirkkalainen,[1] A. A. Clerk,[2] M. J. Woolley,[3] and M. A. Sillanpää[1,*]

[1] *Department of Physics, Aalto University, P.O. Box 15100, FI-00076 AALTO, Finland*
[2] *Department of Physics, McGill University, 3600 rue University, Montréal, Quebec H3A 2T8, Canada*
[3] *School of Engineering and Information Technology, UNSW Canberra, ACT, 2600, Australia*

(Dated: September 6, 2016)

## TWO-TONE, TWO-MODE BACK-ACTION-EVADING MEASUREMENT

### Hamiltonian

The system is composed of one high-$Q$ cavity mode (with annihilation operator $a$) coupled independently to two high-$Q$ mechanical modes (with annihilation operators $b_1$ and $b_2$) via standard radiation-pressure-like couplings [1]. Consequently, its dynamics are well-described by the Hamiltonian (with $\hbar = 1$),

$$H = \omega_a a^\dagger a + \sum_{i=1}^{2} \omega_i b_i^\dagger b_i + \sum_{i=1}^{2} g_i (b_i + b_i^\dagger) a^\dagger a + H_{\text{drive}} + H_{\text{diss}}, \tag{1}$$

where $\omega_a$ and $\omega_i$ are the resonance frequencies of the cavity and mechanical oscillator modes (respectively), and $g_i$ are the single-photon optomechanical coupling rates to these mechanical oscillators.

$H_{\text{diss}}$ accounts for dissipation into Markovian baths with thermal occupations $n_c^T$, $n_1^T$ and $n_2^T$, at rates $\kappa$, $\gamma_1$ and $\gamma_2$ (respectively). The cavity decay rate may be further decomposed as $\kappa = \kappa_{\text{Ei}} + \kappa_{\text{Eo}} + \kappa_{\text{I}}$, where $\kappa_{\text{Ei}}$ and $\kappa_{\text{Eo}}$ are *external* cavity decay rates associated with the in-coupling and out-coupling of microwave fields via transmission lines, and $\kappa_{\text{I}}$ denotes the intrinsic cavity losses.

In order to realize a back-action-evading measurement of a collective quadrature of the two mechanical oscillators with only two tones, the cavity is driven at the frequencies [2],

$$\omega_\pm = \omega_a \pm \frac{\omega_1 + \omega_2}{2}. \tag{2}$$

This driving, with strengths $\mathcal{E}_+$ and $\mathcal{E}_-$, is described by the Hamiltonian contribution

$$H_{\text{drive}} = \left(\mathcal{E}_+^* e^{+i\omega_+ t} + \mathcal{E}_-^* e^{+i\omega_- t}\right) a + \text{H.c.} \tag{3}$$

We assume that the system is in the resolved-sideband regime ($\omega_1, \omega_2 \gg \kappa$), that the mechanical oscillator frequency difference is large compared with the mechanical linewidths ($|\omega_1 - \omega_2| \gg \gamma_1, \gamma_2$), that the system is in the single-photon weak coupling regime ($g_1, g_2 \ll \omega_1, \omega_2$), and that the system is driven with equal strength at both frequencies ($|\mathcal{E}_+| = |\mathcal{E}_-|$). Then its dynamics are well-described by the Hamiltonian [2],

$$H = \Omega(X_+ X_- + P_+ P_-) + 2G(\cos\theta\, X_+ + \sin\theta\, P_+)(a + a^\dagger) + 2G_{\text{mm}}(\cos\theta\, X_- + \sin\theta\, P_-)(a + a^\dagger), \tag{4}$$

where the collective mechanical quadratures ($X_\pm$ and $P_\pm$) are as defined in the main text. The Hamiltonian (4) is specified in an interaction picture defined with respect to the Hamiltonian,

$$H_0 = \omega_a a^\dagger a + \left(\frac{\omega_1 + \omega_2}{2}\right)(b_1^\dagger b_1 + b_2^\dagger b_2). \tag{5}$$

The effective mechanical oscillator frequency in (4) is given by

$$\Omega = \frac{\omega_1 - \omega_2}{2}, \tag{6}$$

and the effective optomechanical coupling in (4) is given by

$$G = \left(\frac{g_1 + g_2}{2}\right)\bar{a}. \tag{7}$$

Here $\bar{a} = \sqrt{n}$ with $n$ being the steady-state photon number in the cavity at *each* of the two drive frequencies, and $\theta$ is the phase of the effective optomechanical coupling. These two quantities are given, in terms of the driving strengths of Eq. (3), by

$$\bar{a}_{\pm} = \bar{a}e^{\pm j\theta} = \frac{-2i\mathcal{E}_{\pm}}{-i(\omega_1+\omega_2)+\kappa}. \tag{8}$$

The optomechanical coupling in (4) arising from the *mismatch* in the single-photon optomechanical coupling rates is

$$G_{\mathrm{mm}} = \left(\frac{g_1 - g_2}{2}\right)\bar{a}, \tag{9}$$

It is henceforth assumed that $|g_1+g_2| \gg |g_1-g_2|$, and we subsequently neglect the mismatch terms in the Hamiltonian (4). This assumption is well-justified both numerically and experimentally. Further, setting $\theta = 0$ yields

$$H = \Omega(X_+X_- + P_+P_-) + 2GX_+(a+a^\dagger), \tag{10}$$

which describes a measurement of the $X_+$ collective mechanical quadrature and corresponds to Eq. (1) of the main text. For varying $\theta$, we can measure the *generalised* collective quadrature $X_+^\theta = \cos\theta\, X_+ + \sin\theta\, P_+$. Clearly, with $\theta = \pi/2$, we measure the collective mechanical quadrature $P_+$.

### Mechanical noise spectra

In order to study the back-action of the measurement, we seek the noise spectra of the collective mechanical quadratures, defined by

$$S_Z[\omega] = \lim_{t\to\infty} 2\,\mathrm{Re}\int_0^{+\infty} d\tau\, e^{i\omega\tau}\langle Z(t+\tau)Z(t)\rangle, \tag{11}$$

where $Z = X_+$ or $P_+$. Note that these spectra *are* symmetric-in-frequency, even though they are not explicitly defined as such. They may be calculated starting from the Heisenberg-Langevin equations corresponding to the Hamiltonian (4) and conventional dissipation into a Markovian thermal bath [3]. Here we shall introduce the *average* mechanical damping rate by

$$\gamma = \frac{\gamma_1+\gamma_2}{2}, \tag{12}$$

and neglect the effects of the asymmetry in the mechanical damping rates. Again, this assumption is well-justified both numerically and experimentally, though a more thorough treatment may be found in Ref. [2]. This assumption leaves us with the system of Heisenberg-Langevin equations,

$$\frac{d}{dt}\vec{X} = \mathbf{A}\cdot\vec{X} + \mathbf{B}\cdot\vec{X}_{\mathrm{in}}, \tag{13}$$

where $\vec{X} = (X_+, P_-, X_-, P_+, X_a, P_a)^T$ is a vector of collective mechanical and cavity quadrature operators, and

$$\vec{X}_{\mathrm{in}} = (X_{+,\mathrm{in}}, P_{-,\mathrm{in}}, X_{-,\mathrm{in}}, P_{+,\mathrm{in}}, X_{a,\mathrm{in}}, P_{a,\mathrm{in}})^T, \tag{14}$$

is a vector of Markovian input noise operators [2, 3]. Neglecting the small effect of $n_1^T \neq n_2^T$ on the form of the input noise terms, the matrices in Eq. (13) are

$$\mathbf{A} = \begin{bmatrix} -\gamma/2 & \Omega & 0 & 0 & 0 & 0 \\ -\Omega & -\gamma/2 & 0 & 0 & 0 & 0 \\ 0 & 0 & -\gamma/2 & \Omega & 0 & 0 \\ 0 & 0 & -\Omega & -\gamma/2 & -2\sqrt{2}G & 0 \\ 0 & 0 & 0 & 0 & -\kappa/2 & 0 \\ -2\sqrt{2}G & 0 & 0 & 0 & 0 & -\kappa/2 \end{bmatrix}, \tag{15a}$$

$$\mathbf{B} = \left[\begin{array}{c|c} \sqrt{\gamma(n_1^T+n_2^T+1)/2}\,\mathbf{I}_4 & \mathbf{0}_{42} \\ \hline \mathbf{0}_{24} & \sqrt{\kappa(2n_c^T+1)/2}\,\mathbf{I}_2 \end{array}\right], \tag{15b}$$

where $\mathbf{0}_{mn}$ denotes the $m \times n$ zero matrix and $\mathbf{I}_{nn}$ denotes the $n \times n$ identity matrix.

Now the steady-state, symmetrically-ordered covariance matrix $\mathbf{V}$ describing the steady-state of Eq. (13) follows from solution of the Lyapunov equation,

$$\mathbf{AV} + \mathbf{VA}^T = -\mathbf{BB}^T. \tag{16}$$

Subsequently, we can calculate the correlation functions in the integrand of (11) using the quantum regression theorem [7], and the spectra for the collective mechanical quadratures of interest follow as

$$S_{X_+}[\omega] = \frac{1}{2}(1 + n_1^T + n_2^T)S_0[\omega], \tag{17a}$$

$$S_{P_+}[\omega] = \frac{1}{2}\left[1 + n_1^T + n_2^T + 4C\frac{\kappa^2}{\kappa^2 + 4\Omega^2}(2n_{\rm c}^T + 1)\right]S_0[\omega], \tag{17b}$$

as quoted in Eqs. (2)-(3) of the main text. The *cooperativity* has been introduced as

$$C = \frac{4G^2}{\gamma\kappa}, \tag{18}$$

and $S_0[\omega]$ denotes the spectrum corresponding to a sum of two Lorentzians centred at $\omega = \pm\Omega$ and with linewidths $\gamma$,

$$S_0[\omega] = \frac{2\gamma}{\gamma^2 + 4(\omega - \Omega)^2} + \frac{2\gamma}{\gamma^2 + 4(\omega + \Omega)^2}. \tag{19}$$

Here $S_0[\omega]$ has been normalised such that $(2\pi)^{-1}\int_{-\infty}^{+\infty} d\omega\, S_0[\omega] = 1$. Note that the spectra quoted here, as well as those quoted henceforth, may also be calculated from the Fourier-transformed Heisenberg-Langevin equations in the usual manner [4].

It is useful to define an *effective occupation* for each collective mechanical quadrature via

$$n_Z + \frac{1}{2} \equiv \langle Z^2\rangle = \frac{1}{2\pi}\int_{-\infty}^{+\infty} d\omega\, S_Z[\omega], \tag{20}$$

such that $n_Z$ corresponds to the integrated noise spectral density minus a contribution from the quantum zero-point fluctuations.

**Cavity output spectrum**

The spectrum analyzer measures the symmetrized noise spectral density of the voltage at the output of the amplifier [5]. Since the amplifier is the dominant source of imprecision noise here, and we are ultimately interested in the output photon flux, it suffices to calculate the normally-ordered spectrum. First, we calculate the normally-ordered *intracavity* noise spectrum, defined by

$$S_a[\omega] = \lim_{t\to\infty} 2\,\mathrm{Re}\int_0^{+\infty} d\tau e^{i\omega\tau}\langle a^\dagger(t+\tau)a(t)\rangle. \tag{21}$$

It may be calculated using the quantum regression theorem [7], and we find

$$S_a[\omega] = \frac{16G^2}{\kappa^2 + 4\omega^2}S_{X_+}[\omega] + \frac{4\kappa}{\kappa^2 + 4\omega^2}n_{\rm c}^T. \tag{22}$$

The cavity *output* spectrum, with the output field $a_{\rm out}(t)$ defined in the standard manner, follows as [3]

$$S_{\rm out}[\omega] = \lim_{t\to\infty} 2\,\mathrm{Re}\int_0^{+\infty} d\tau e^{i\omega\tau}\langle a_{\rm out}^\dagger(t+\tau)a_{\rm out}(t)\rangle = \kappa_{\rm Eo}S_a[\omega], \tag{23}$$

where we recall that $\kappa_{\rm Eo}$ is the cavity decay rate associated with out-coupling of the microwave field. Using Eq. (22), it follows that

$$S_{\rm out}[\omega] = \frac{16G^2\kappa_{\rm Eo}}{\kappa^2 + 4\omega^2}S_{X_+}[\omega] + \frac{4\kappa\kappa_{\rm Eo}}{\kappa^2 + 4\omega^2}n_c^T. \tag{24}$$

The output photon *flux* follows as the integrated cavity output spectrum,

$$n_{\mathrm{out}} \equiv \frac{1}{2\pi}\int_{-\infty}^{+\infty} d\omega\, S_{\mathrm{out}}[\omega] = \kappa_{\mathrm{Eo}} C \frac{4\gamma\kappa}{\kappa^2+4\Omega^2}\frac{1}{2}(n_1^T + n_2^T + 1) + \kappa_{\mathrm{Eo}} n_{\mathrm{c}}^T, \tag{25}$$

as quoted in Eq. (4) of the main text under the assumption $n_{\mathrm{c}}^T = 0$. In calculating the first term of the result in quoted in Eq. (25) we have made the replacement $\omega^2 \to \Omega^2$ in the coefficient of $S_{X_+}[\omega]$ in Eq. (24), based on the assumption that the cavity linewidth greatly exceeds the mechanical linewidths ($\kappa \gg \gamma$).

### Amplified cavity output spectrum

The cavity output field is subject to phase-insensitive amplification prior to detection at the spectrum analyzer. Therefore, the measured output field follows from the cavity output field as [4, 8]

$$c(t) = \sqrt{A}a_{\mathrm{out}}(t) + \sqrt{A-1}h^\dagger(t), \tag{26}$$

where $A$ is the amplifier gain, and $h(t)$ is the amplifier input noise operator having the correlation function,

$$\lim_{t\to\infty}\langle h(t+\tau)h^\dagger(t)\rangle = (n_{\mathrm{amp}}+1)\delta(\tau), \tag{27}$$

where $n_{\mathrm{amp}}$ denotes the thermal noise of the amplifier. The required spectrum is then

$$S_c[\omega] = \lim_{t\to\infty} 2\,\mathrm{Re}\int_0^{+\infty} d\tau e^{i\omega\tau}\langle c^\dagger(t+\tau)c(t)\rangle. \tag{28}$$

Using Eqs. (23), (26) and (27), it follows that

$$S_c[\omega] = A\kappa_{\mathrm{Eo}} S_a[\omega] + (A-1)(n_{\mathrm{amp}}+1). \tag{29}$$

Substituting Eq. (22) into Eq. (29) we find

$$S_c[\omega] = \frac{16A\kappa_{\mathrm{Eo}}G^2}{\kappa^2+4\omega^2} S_{X_+}[\omega] + \frac{8A\kappa_{\mathrm{Eo}}\kappa}{\kappa^2+4\omega^2} n_c^T + (A-1)(n_{\mathrm{amp}}+1). \tag{30}$$

The measured noise spectrum contains a filtered version of the measured mechanical noise spectrum (first term), a filtered contribution from the thermal occupation of the cavity mode (second term), and a background noise floor due to the thermal noise of the amplifier (third term). Since the cavity linewidth is much larger than the mechanical linewidth, the cavity output faithfully reproduces the mechanical noise spectrum.

### Imprecision noise

Rearranging Eq. (30), we are led to introducing the measurement imprecision noise spectrum, $S_{X_+}^{\mathrm{imp}}[\omega]$, by

$$\frac{\kappa^2+4\omega^2}{16A\kappa_{\mathrm{Eo}}G^2} S_{\mathrm{c}}[\omega] = S_{X_+}[\omega] + S_{X_+}^{\mathrm{imp}}[\omega], \tag{31}$$

such that we have

$$S_{X_+}^{\mathrm{imp}}[\omega] = \frac{\kappa}{2G^2} n_{\mathrm{c}}^T + (n_{\mathrm{amp}}+1)\frac{A-1}{A}\frac{\kappa^2+4\omega^2}{16\kappa_{\mathrm{Eo}}G^2}. \tag{32}$$

Assuming that the amplifier gain is large we can approximate $(A-1)/A \to 1$ in Eq. (32). Further, assuming that the cavity damping is dominated by the out-coupling of the microwave field to the transmission line (i.e., $\kappa \sim \kappa_{\mathrm{Eo}}$) and rewriting the result in terms of the cooperativity, we obtain

$$S_{X_+}^{\mathrm{imp}}[\omega] = \frac{2/\gamma}{C} n_{\mathrm{c}}^T + \frac{1/\gamma}{4C}\frac{\kappa^2+4\omega^2}{\kappa^2}(n_{\mathrm{amp}}+1). \tag{33}$$

This result leads us to define an imprecision noise *in quanta* for $\omega \sim \pm\Omega$ (within a mechanical linewidth) by

$$n_{X_+}^{\text{imp}} \equiv \frac{\gamma}{2} S_{X_+}^{\text{imp}}[\pm\Omega], \tag{34}$$

which yields Eq. (5) of the main text. This definition is motivated by observing that for the unperturbed ($X_+$) mechanical noise spectrum given by Eq. (17a) we have

$$n_{X_+} + \frac{1}{2} = \langle X_+^2 \rangle = \frac{1}{2\pi} \int_{-\infty}^{+\infty} S_{X_+}[\omega] d\omega = \frac{\gamma}{2} S_{X_+}[\pm\Omega]. \tag{35}$$

In general, the effective occupation thus defined may be decomposed as

$$n_{X_+} = n_{X_+}^{T} + n_{X_+}^{\text{BA}} + n_{X_+}^{\text{imp}}, \tag{36}$$

with $n_{X_+}^T = (n_1^T + n_2^T)/2$ representing thermal fluctuations, and $n_{X_+}^{\text{BA}}$ representing spurious back-action onto the measured quadrature including technical heating.

The result of Eq. (33) can be discussed in the context of imprecision back-action uncertainty relations [4]. Recall from Eq. (17b) that the frequency-dependent backaction onto the conjugate quadrature (i.e., $P_+$, assuming that $X_+$ is measured) is

$$S_{P_+}^{\text{ba}}[\omega] = 4C(2n_{\text{c}}^T + 1)\frac{\kappa^2}{\kappa^2 + 4\Omega^2}\left[\frac{\gamma}{\gamma^2 + 4(\omega - \Omega)^2} + \frac{\gamma}{\gamma^2 + 4(\omega + \Omega)^2}\right]. \tag{37}$$

If we set $n_{\text{c}}^T = n_{\text{amp}} = 0$ and $\omega = \pm\Omega$ in Eqs. (33) and (37), then we have

$$S_{X_+}^{\text{imp}}[\Omega] = \frac{1/\gamma}{4C}\frac{\kappa^2 + 4\Omega^2}{\kappa^2}, \tag{38a}$$

$$S_{P_+}^{\text{ba}}[\Omega] = 4C\frac{\kappa^2}{\kappa^2 + 4\Omega^2}\frac{1}{\gamma}, \tag{38b}$$

and consequently, their product is

$$S_{X_+}^{\text{imp}}[\Omega] \cdot S_{P_+}^{\text{ba}}[\Omega] = 1/\gamma^2. \tag{39}$$

Using Eq. (34), this leads to the imprecision back-action product quoted in the main text. We note that if one rescales $S_{P_+}^{\text{ba}}$ so that it is the spectral density of the effective force fluctuations driving the $P_+$ mode, then Eq. (39) takes the form of a standard imprecision-backaction constraint on spectral densities (with a lower bound of 1/4).

## ONE-TONE, TWO-MODE OPTOMECHANICAL COOLING

### Hamiltonian

Again we consider the system described by the Hamiltonian (1), but now with the blue sideband drive turned off. That is, the driving terms (3) now have $\mathcal{E}_+ = 0$. The Hamiltonian (1) now becomes [9]

$$H = \Omega(X_+X_- + P_+P_-) + \sqrt{2}G\cos\theta(X_+X_a + P_+P_a) + \sqrt{2}G\sin\theta(P_+X_a + X_+P_a), \tag{40}$$

where the effective optomechanical coupling in (40) is now

$$G = \left(\frac{g_1 + g_2}{2}\right)\bar{a}_-, \tag{41}$$

and we have neglected mismatch terms in the Hamiltonian, as was done for the Hamiltonian (10). Setting $\theta = 0$ without loss of generality, the Hamiltonian may be rewritten in terms of annihilation and creation operators as

$$H = \Omega(b_1^\dagger b_1 - b_2^\dagger b_2) + G[a(b_1^\dagger + b_2^\dagger) + \text{H.c.}]. \tag{42}$$

In this form it is clear, provided the cavity damping rate exceeds the mechanical damping rates ($\kappa \gg \gamma$), that the system dynamics will correspond to independent detuned optomechanical cooling of two independent mechanical modes [1, 9].

**Steady-state**

The standard optomechanical cooling analysis [1, 10, 11] shows that the mechanical oscillator modes will be subject to an optomechanical damping and an optomechanical frequency shift, given by

$$\Gamma_{\mathrm{opt}} = \frac{4G^2\kappa}{\kappa^2 + 4\Omega^2}, \tag{43a}$$
$$\delta\Omega_{\mathrm{opt}} = \frac{4G^2\Omega}{\kappa^2 + 4\Omega^2}. \tag{43b}$$

respectively. Neglecting the small frequency shift it follows that the steady-state occupation of the mechanical oscillator modes, $n_i \equiv \langle b_i^\dagger b_i \rangle$, are then

$$n_i = n_i^T \frac{\gamma_i}{\gamma_i + \Gamma_{\mathrm{opt}}} + n_{\mathrm{c}}^T \frac{\Gamma_{\mathrm{opt}}}{\gamma_i + \Gamma_{\mathrm{opt}}} \to n_i^T \frac{\gamma_i}{\gamma_i + \Gamma_{\mathrm{opt}}}, \tag{44}$$

where the limit follows in the usual case that $n_{\mathrm{c}}^T = 0$ to a good approximation.

**Cavity output spectrum**

As in the case of a back-action-evading measurement, we are interested in the output photon flux. This can be obtained from the normally-ordered cavity output spectrum given by Eq. (23). Writing out the Heisenberg-Langevin equations corresponding to the Hamiltonian (40) and solving for the correlation functions using the quantum regression theorem leads to the spectrum

$$S_{\mathrm{out}}[\omega] = \frac{1}{2}(n_1 + n_2)\frac{8G^2\kappa_{\mathrm{Eo}}}{\kappa^2 + 4\omega^2}\left[\frac{2\bar{\gamma}}{\bar{\gamma}^2 + 4(\omega - \bar{\Omega})^2} + \frac{2\bar{\gamma}}{\bar{\gamma}^2 + 4(\omega + \bar{\Omega})^2}\right] + \frac{4\kappa\kappa_{\mathrm{Eo}}}{\kappa^2 + 4\omega^2} n_{\mathrm{c}}^T, \tag{45}$$

where the effective mechanical damping rate and frequency (shifted by the optomechanical coupling) are given by

$$\bar{\gamma} = \gamma + \Gamma_{\mathrm{opt}}, \tag{46a}$$
$$\bar{\Omega} = \Omega + \delta\Omega_{\mathrm{opt}}, \tag{46b}$$

respectively, and $n_i$ are the steady-state mechanical occupations given by Eq. (44). In contrast to the back-action-evading result in Eq. (24), the cavity output spectrum is insensitive to the mechanical quantum zero-point fluctuations.

The output photon flux is again given by the integrated cavity output spectrum. Using Eq. (45), making the replacement $\omega \to \bar{\Omega}$ in the coefficient of the first term (assuming $\kappa \gg \gamma$), and integrating we find

$$n_{\mathrm{out}} = \frac{1}{2\pi}\int_{-\infty}^{+\infty} d\omega\, S_{\mathrm{out}}[\omega] = (n_1^T + n_2^T)\frac{\gamma}{\gamma + \Gamma_{\mathrm{opt}}}\frac{4G^2\kappa_{\mathrm{Eo}}}{\kappa^2 + 4\bar{\Omega}^2} + \kappa_{\mathrm{Eo}} n_{\mathrm{c}}^T. \tag{47}$$

The result in Eq. (47) can be further simplified by noting that while we can certainly have $\Gamma_{\mathrm{opt}} \gg \gamma$, we are typically operating in a parameter regime such that $\delta\Omega_{\mathrm{opt}} \ll \Omega$, and so henceforth the optomechanical frequency shift shall be neglected (i.e., $\bar{\Omega} \to \Omega$). Further, expressing the optomechanical damping rate in terms of the cooperativity, we obtain a sublinear dependence of the output photon flux on the cooperativity:

$$n_{\mathrm{out}} = C\frac{\gamma\kappa\kappa_{\mathrm{Eo}}}{4\Omega^2 + \kappa^2(C+1)}(n_1^T + n_2^T) + \kappa_{\mathrm{Eo}} n_{\mathrm{c}}^T. \tag{48}$$

In the low-cooperativity limit ($C \ll 1$) this becomes

$$n_{\mathrm{out}} = C\frac{\gamma\kappa\kappa_{\mathrm{Eo}}}{\kappa^2 + 4\Omega^2}(n_1^T + n_2^T) + \kappa_{\mathrm{Eo}} n_{\mathrm{c}}^T. \tag{49}$$

Eq. (49) is half the back-action-evading result given by Eq. (25), but without a contribution from the mechanical quantum zero-point fluctuations. This is to be expected since the input microwave power in the cooling configuration is half the input power in the back-action-evading measurement configuration.

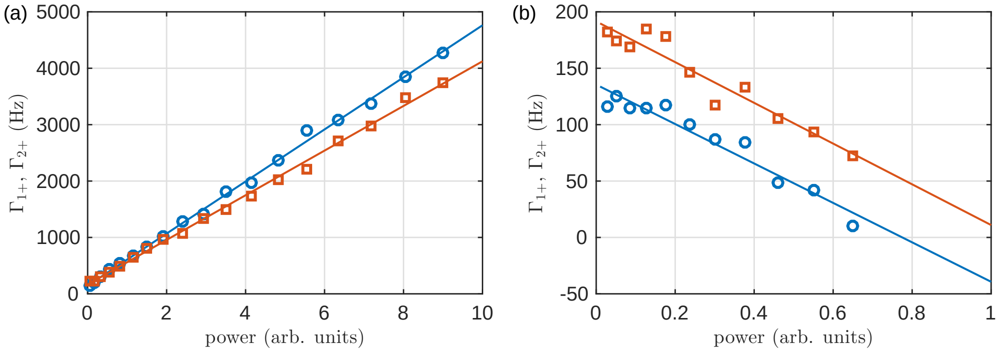


Figure 1. *Calibration of* $g_1/g_2$. Total damping rate of mechanical oscillators 1 (red squares) and 2 (blue circles) as a function of microwave pump power, with linear fits. (a) Red-detuned pump. (b) Blue-detuned pump.

## OPTOMECHANICAL COUPLING STRENGTHS

The ratio $g_1/g_2$ of single-photon optomechanical couplings of the two mechanical oscillators can be calibrated using standard optomechanical cooling [1, 10, 11]. We used a single pump either at the red-detuned side with $\omega_- = \omega_a - (\omega_1 + \omega_2)/2$, or at the blue-detuned side with $\omega_+ = \omega_a + (\omega_1 + \omega_2)/2$. These pump frequencies are hence the same as in the actual BAE experiment, but only a single tone is applied at a time. Since the pumps are not at the sideband resonance for either oscillator, the optomechanical cooling and heating is smaller than in the standard, resonant case. With the red-detuned (blue-detuned) pump the damping is increased (decreased), and the total damping rate of the oscillators in these cases are [10, 11]

$$\Gamma_{\mp} = \gamma \pm \frac{4G^2\kappa}{\kappa^2 + 4(\omega_{\mp} - \omega_a \pm \omega_i)^2} . \tag{50}$$

In both cases, the damping depends linearly on the pump power, and quadratically on the single-photon coupling $g_i$. The ratio $g_1/g_2$ is hence given by the square root of the ratio of slopes of damping plotted as a function of input microwave power, and the ratio should be the same with either detuning. We show the analysis in Fig. 1. From Fig. 1(a) we obtain $g_1/g_2 \simeq 0.926 \pm 0.013$, whereas from Fig. 1(b) we find $g_1/g_2 \simeq 1.02 \pm 0.10$. At the blue side, the system becomes unstable when the damping approaches zero, which limits the available dynamic range and the statistics in the blue case. We calculate the average of the values from (a) and (b) weighted with the fit uncertainties, and obtain the final number $g_1/g_2 \simeq 0.94 \pm 0.02$.

The back-action evading nature of the two-tone measurement only strictly holds if the single-photon couplings and mechanical damping rates are equal. If $g_1 \neq g_2$, adverse terms appear in the Hamiltonian of Eq. (10), and dissimilar dampings $\gamma_1 \neq \gamma_2$ results in the corresponding equations of motion to lose the symmetry [2]. However, for our experimental parameters we expect negligible degradation of the BAE for measurement strengths up to $C \lesssim 10$. At the highest power used, the expected residual back-action on the measured $X_+$ quadrature is $\sim 2$ quanta, much smaller than the quantum back-action $n_{\mathrm{BA,q}} \approx 63$. In the present experiment, this residual back-action is also negligible compared to the effective temperatures $n_i^T$.

* mika.sillanpaa@aalto.fi

[1] M. Aspelmeyer, T. J. Kippenberg, and F. Marquardt, *Rev. Mod. Phys.* **86**, 1391 (2014).
[2] M. J. Woolley and A. A. Clerk, *Phys. Rev. A* **87**, 063846 (2013).
[3] D. F. Walls and G. J. Milburn, *Quantum Optics*, Springer, 2008.
[4] A. A. Clerk, M. H. Devoret, S. M. Girvin, F. Marquardt, and R. J. Schoelkopf, *Rev. Mod. Phys.* **82**, 1155 (2010).
[5] A. J. Weinstein, C. U. Lei, E. E. Wollman, J. Suh, A. Metelmann, A. A. Clerk, and K. C. Schwab, *Phys. Rev. X* **4**, 041003 (2014).
[6] C. W. Gardiner and P. Zoller, *Quantum Noise*, Springer, 2004.
[7] H.-P. Breuer and F. Petrucionne, *The Theory of Open Quantum Systems*, Oxford University Press, 2002.
[8] C. M. Caves, *Phys. Rev. D* **26**, 1817 (1982).

[9] M. J. Woolley and A. A. Clerk, *Phys. Rev. A* **89**, 063805 (2014).
[10] I. Wilson-Rae, N. Nooshi, W. Zwerger, and T. J. Kippenberg, *Phys. Rev. Lett.* **99**, 093901 (2007).
[11] F. Marquardt, J. P. Chen, A. A. Clerk, and S. M. Girvin, *Phys. Rev. Lett.* **99**, 093902 (2007).
